# Supplementary material for: When Measurement Constraints Favor Quantum Computational Sensing for Stealthy Power-Grid Attack Detection
Source: arXiv:2609.10606 source file (2026-09-08)
Supplement: Supplementary file 1 [file cross_sensor_interaction.tex]

\section{Cross-Sensor Quantum Interaction Budget}
\label{app:interaction-budget}

To quantify the cost of enforcing local processing, we compare independent,
pairwise/tree-structured, chain-structured, and fully joint quantum processing
on case14 CTA under the same finite-shot protocol.

\begin{table}[h]
\centering
\caption{AP versus cross-sensor quantum interaction (case14 CTA).}
\label{tab:interaction-full}
\begin{tabular}{lccccccc}
\toprule
Architecture & 10 & 50 & 100 & 500 & 1000 & 5000 & exact \\
\midrule
Independent ($Q{=}0, N{=}1$)
& 0.539 & 0.604 & 0.609 & 0.685 & 0.697 & 0.706 & 0.710 \\
Pairwise/tree-joint (QutritTTN)
& 0.890 & 0.979 & 0.986 & 0.991 & 0.992 & 0.993 & 0.992 \\
Chain-joint (QutritMPS)
& 0.845 & 0.971 & 0.980 & 0.993 & 0.994 & 0.995 & 0.995 \\
Fully-joint oracle ($\mathrm{SU}(3^5)$)
& 0.938 & 0.984 & 0.987 & 0.988 & 0.990 & 0.990 & 0.990 \\
\bottomrule
\end{tabular}
\end{table}

Allowing even limited cross-sensor quantum interaction produces a large gain:
at 10 shots, the pairwise and chain-structured models already exceed the exact
independent baseline. This indicates that CTA contains genuinely spatial
information distributed across sensors, and that purely local processing leaves
some of that structure inaccessible before measurement.

We nevertheless retain local QCS as the deployment architecture because
pairwise and fully joint models require coherent access across physically
separated sensor sites. The joint variants are therefore treated as oracle
upper bounds that quantify the potential value of distributed quantum
interaction rather than as deployment assumptions.
