# Supplementary material for: When Measurement Constraints Favor Quantum Computational Sensing for Stealthy Power-Grid Attack Detection
Source: arXiv:2609.10606 source file (2026-09-08)
Supplement: Supplementary file 2 [file interleaving_depth.tex]

\section{Interleaving Depth: Extended Sweep}
\label{app:interleaving-depth}

% \Cref{sec:rq2-interleaved} reports the headline exact-shot numbers for
% $N\in\{1,2,4,8,10,16\}$ on case14 CTA; here we give the full shot-dependent picture and training time.

\begin{table}[h]
\centering
\caption{Interleaved-QCS, AP by interleaving depth and shot budget
(case14, CTA, $n{=}1020$).}
\label{tab:interleave-full}
\begin{tabular}{lccccc}
\toprule
$N$ & 10 shots & 100 shots & 1000 shots & exact & Train time \\
\midrule
1 (post-hoc)              & 0.558 & 0.634 & 0.686 & 0.710 & $\sim$150s \\
2                          & 0.628 & 0.746 & 0.814 & 0.821 & 155s \\
4                          & 0.781 & 0.885 & 0.914 & 0.919 & 291s \\
8                          & 0.890 & 0.960 & 0.979 & 0.980 & 547s \\
10                         & 0.901 & 0.961 & 0.983 & 0.985 & 705s \\
16                         & 0.925  & 0.961 & 0.961 & 0.966 & 14298s \\
\bottomrule
\end{tabular}
\end{table}

Two findings shape our choice of $N{=}10$ as the paper's headline
architecture rather than a larger value. First, returns diminish smoothly
before $N{=}10$: $N{=}4\to8$ (a 100\% increase in depth) buys $+0.061$ exact
AP, while $N{=}8\to10$ (a 25\% increase) buys only $+0.005$ -- consistent
with an information-theoretic argument that once nearly all extractable
information is being captured, additional interleaving has less left to
gain. Second, $N{=}16$ is not merely diminishing but \emph{negative}
returns: at $\sim$20$\times$ $N{=}10$'s training cost (14298s vs.\ 705s,
itself a super-linear -- not merely linear-in-$N$ -- blowup, most likely
from matrix-exponential backward-pass cost compounding over longer composed
chains), it reaches only $0.966$, below $N{=}10$'s $0.985$. This mirrors the
same optimization-difficulty pattern: chaining more sequential trainable
quantum operations makes optimization harder, not easier, past some depth.
We therefore treat $N\sim8$--$10$ as a practical sweet spot specific to this
hardware/optimizer combination.

\paragraph{The $N=1$ limit and interleaving depth}
% \label{app:interleaving-depth}

We parameterize Interleaved-QCS by the number of sensing/control stages
$  N\in\{1,2,4,8,10,16\}.$
For a fixed sensing duration, increasing $N$ divides the field interaction into
shorter intervals separated by learned coherent controls.
The $N=1$ model is the degenerate limit of the same architecture: the field
interaction completes before a single trainable unitary is applied. It
therefore represents post-sensing control rather than genuine interleaving,
while keeping the same sensor Hilbert space and final measurement structure.
This provides a direct ablation of whether acting \emph{during} sensing offers
additional value beyond applying a trainable unitary only after sensing.
We verify that the implemented $N=1$ construction matches the corresponding
post-sensing-control circuit to numerical precision. Larger $N$ is not assumed
to be uniformly preferable; performance and optimization behavior are evaluated
empirically.

\paragraph{Construction checks:} Because a static field over a
fixed sensing window decomposes exactly,
$\exp(L\tau_s) = \exp(L\tau_s/N)^N$ for any $N$, Interleaved-QCS's
per-sample physics sub-propagator is precomputed once per sample/sensor with
zero discretization error (not an approximation of continuous interleaving).
We verified this construction two ways before trusting any result built on
it: (1) $N{=}1$ reproduces the base simulator's \texttt{evolve\_rho} exactly
(0.0 deviation); (2) the general $N$-step implementation evaluated at
$N{=}1$ exactly matches the original single-measurement implementation
given identical parameters (0.0 deviation) -- confirming the interleaved
architecture correctly generalizes the post-hoc case as its $N{=}1$
special case, rather than being a different, incomparable model.
