# Supplementary material for: When Measurement Constraints Favor Quantum Computational Sensing for Stealthy Power-Grid Attack Detection
Source: arXiv:2609.10606 source file (2026-09-08)
Supplement: Supplementary file 3 [file qcs_architecture.tex]

\section{Additional Quantum-Sensing Architecture Details}
\label{app:architecture-details}

This appendix expands on the architectural choices summarized in
\Cref{sec:architecture}, including the role of interleaving, the $N=1$ limit,
classicalize-then-requantize baselines, joint multi-sensor processing, and
oracle evidence-channel combinations.

\subsection{Why interleave coherent control with sensing?}
\label{app:interleaving-rationale}

The distinction between QCS and a conventional variational readout is not
simply the presence of a trainable unitary, but \emph{when} that control acts.
If sensing is completed first, a subsequent unitary can only reorganize
information already encoded in the final sensor state before measurement.
Interleaved QCS instead applies coherent control while information about the
field is accumulating:
\[
    \rho_{k+1}
    =
    U_{\theta_k}
    \mathcal{E}_{B,\Delta t}(\rho_k)
    U_{\theta_k}^{\dagger}.
\]
The learned controls can therefore modify the sensing trajectory itself and
shape which task-relevant information becomes accessible in the final
measurement. This is the central mechanism underlying QCS
\citep{khan2026qcs} and is closely related to controlled and adaptive
quantum-metrology protocols
\citep{rlmetrology2021,adaptivecircuitmetrology2020,
programmablesensors2022}.

We do not assume that interleaving necessarily reaches the quantum
Cram\'er--Rao limit. Rather, it provides a trainable mechanism for converting
information present in the physical quantum evolution into a task-specific
measurement. The QFI/CFI analysis in our experiments separately examines how
much information is available in principle versus how much the trained model
actually extracts.

\subsection{The $N=1$ limit and interleaving depth}
\label{app:interleaving-depth}

We parameterize Interleaved-QCS by the number of sensing/control stages
\[
    N\in\{1,2,4,8,10,16\}.
\]
For a fixed sensing duration, increasing $N$ divides the field interaction into
shorter intervals separated by learned coherent controls.
The $N=1$ model is the degenerate limit of the same architecture: the field
interaction completes before a single trainable unitary is applied. It
therefore represents post-sensing control rather than genuine interleaving,
while keeping the same sensor Hilbert space and final measurement structure.
This provides a direct ablation of whether acting \emph{during} sensing offers
additional value beyond applying a trainable unitary only after sensing.
We verify that the implemented $N=1$ construction matches the corresponding
post-sensing-control circuit to numerical precision. Larger $N$ is not assumed
to be uniformly preferable; performance and optimization behavior are evaluated
empirically.

\subsection{Classicalize-then-requantize ablation}
\label{app:vqc-flattened}

A different QML pipeline first converts the NV density matrix into classical
features and subsequently encodes those features into a separate parameterized
quantum circuit. One representation concatenates the real and imaginary
entries of the qutrit density matrix,
\[
    x(\rho)
    =
    [
    \operatorname{Re}(\rho_{11}),\ldots,\operatorname{Re}(\rho_{33}),
    \operatorname{Im}(\rho_{11}),\ldots,\operatorname{Im}(\rho_{33})
    ],
\]
yielding 18 real-valued inputs before re-encoding.

We retain this only as an ablation because it answers a different QML
question. The physical quantum state is first classicalized and then encoded
into a new quantum system. In QCS, by contrast, the computational state
\emph{is the physical sensor state itself}: learning acts directly on the
quantum information generated by sensing.

This distinction is important for the interpretation of our results. A
classicalize-then-requantize model evaluates whether a quantum classifier can
process classical sensor features; QCS evaluates whether trainable quantum
processing is useful \emph{before} the physical sensor state is converted into
classical data.

\subsection{Tomography and exact-state oracle}
\label{app:reconstruction}

A general qutrit density matrix has eight independent real degrees of freedom.
Recovering these requires measurements in multiple bases over repeated state
preparations. Tomography therefore provides substantially richer classical
information than a single fixed readout, but incurs a correspondingly larger
physical measurement cost.

Our simulator also exposes the exact density matrix $\rho$. This quantity is
never directly available from a real sensor and is therefore used only to
construct oracle upper bounds and diagnostic comparisons. All results based on
exact $\rho$, exact physical fields, or equivalent simulator-internal
quantities are labeled as oracle results and are excluded from deployment
recommendations.

\subsection{Local versus joint multi-sensor quantum processing}
\label{app:interaction-budget}

The deployable architecture processes each spatially separated NV sensor
locally and fuses only classical outputs:
\[
    \rho_i
    \rightarrow
    \mathrm{QCS}_i
    \rightarrow
    m_i,
    \qquad
    [m_1,\ldots,m_K]
    \rightarrow
    f_{\mathrm{classical}}
    \rightarrow
    \hat y.
\]
This requires neither shared entanglement nor coherent quantum communication
between transmission-line sensor sites.

For diagnostic purposes, we additionally consider a joint model,
\[
    \rho_1\otimes\cdots\otimes\rho_K
    \longrightarrow
    U_{\theta}^{\mathrm{joint}}
    \longrightarrow
    M,
\]
which assumes coherent access to all sensor states. We treat this only as an
oracle upper bound: its purpose is to estimate the potential value of
cross-sensor quantum interaction, not to define the deployment architecture.

This distinction also clarifies the relation to distributed entangled sensing
approaches \citep{zhuang2019slaen,xia2020variational,nader2026triplelayer}.
Those architectures study the value of shared quantum resources across remote
sensors; our primary question is how far task-specific local QCS can go without
requiring such infrastructure.

\subsection{Multi-sensor fusion versus evidence-channel fusion}
\label{app:evidence-fusion}

Multi-sensor fusion and evidence-channel fusion are distinct operations.
Multi-sensor fusion combines the same kind of physical observation across
multiple NV locations. Evidence-channel fusion instead combines heterogeneous
sources such as SCADA telemetry, reported-versus-physical discrepancy, and the
physical NV state.

We therefore evaluate two ensemble variants. The \textbf{oracle ensemble}
combines SCADA with channels that may use simulator-internal information,
including exact-state or exact-discrepancy quantities. It represents an upper
bound on what perfectly accessible heterogeneous evidence could achieve and is
not treated as deployable.

The \textbf{realistic ensemble} contains only channels accessible under the
stated sensing model through finite physical measurements and conventional
telemetry. The performance gap between the two ensembles is itself informative:
it quantifies how much useful information exists in the physical model but is
not accessible through the realistic measurement interface.

All oracle-derived channels are explicitly identified throughout the paper.
