# Supplementary material for: When Measurement Constraints Favor Quantum Computational Sensing for Stealthy Power-Grid Attack Detection
Source: arXiv:2609.10606 source file (2026-09-08)
Supplement: Supplementary file 4 [file qutrit_ablation.tex]

\section{Qutrit Architecture Ablations}
\label{app:qutrit-ablation}

\subsection{SU(2) vs.\ SU(3): does the third level matter?}
We restrict Interleaved-QCS's ($N{=}1$) trainable unitary to the Gell-Mann
generators $\lambda_1,\lambda_2,\lambda_3$ (an $\SU(2)$ subalgebra acting
only on the $\{\ket{-1},\ket{0}\}$ subspace, leaving the $\ket{+1}$
population provably frozen -- verified to exactly $0.0$ deviation) and
compare against the full $\SU(3)$ circuit, case14, same
seed/split/scenarios.

\begin{table}[h]
\centering
\caption{$\SU(2)$ vs.\ $\SU(3)$ control at $N{=}1$, exact-shot AP (case14).}
\label{tab:su2-su3}
\begin{tabular}{lcccc}
\toprule
 & Standard FDIA & BDD-stealth & Statistical-stealth & CTA \\
\midrule
$\SU(2)$ & 0.484 & 0.479 & 0.509 & 0.581 \\
$\SU(3)$ & 0.519 & 0.499 & 0.533 & 0.710 \\
$\Delta$ ($\SU(3)-\SU(2)$) & 0.035 & 0.020 & 0.023 & \textbf{0.129} \\
\bottomrule
\end{tabular}
\end{table}

The pattern mirrors \Cref{sec:results-rq1}'s observability hierarchy one
level down in the architecture: the third level costs almost nothing on the
easy, discrepancy-dominated cyber-only attacks and is specifically useful
on CTA, the one attack where the fine-grained physical state is the only
surviving signal. This rules out ``depth/expressivity doesn't matter'' as
the reason Interleaved-QCS underperforms classical readout at $N{=}1$  ; the qutrit-vs-qubit choice matters exactly where
we would expect it to, it just is not sufficient by itself to close the gap
to tomography.

\subsection{Local vs.\ global parameterization, and circuit depth}
We compare four $N{=}1$ (post-hoc) variants: Global (parameters shared
across all sensors) vs.\ Local (independent per-sensor parameters)
$\times$ $n_{\rm layers} \in \{2, 4\}$.

\begin{table}[h]
\centering
\caption{Robustness of the post-hoc negative result to architecture choice
(case14, CTA).}
\label{tab:local-global}
\begin{tabular}{lcccc}
\toprule
Variant & Params & Train time & AP (exact) & AP (1000 shots) \\
\midrule
Global, $n_{\rm layers}{=}2$ (baseline) & 32  & 152s  & 0.716 & 0.698 \\
Global, $n_{\rm layers}{=}4$            & 48  & 1690s & 0.651 (worse) & 0.654 \\
Local, $n_{\rm layers}{=}2$             & 96  & 150s  & 0.704 & 0.681 \\
Local, $n_{\rm layers}{=}4$             & 176 & 290s  & 0.695 & 0.687 \\
\bottomrule
\end{tabular}
\end{table}

None of the three more expressive variants beats the shallow global
baseline; the deeper global circuit is actively worse, consistent with
optimization difficulty rather than capacity limitation.
