# Supplementary material for: When Measurement Constraints Favor Quantum Computational Sensing for Stealthy Power-Grid Attack Detection
Source: arXiv:2609.10606 source file (2026-09-08)
Supplement: Supplementary file 5 [file sensor_count_scale.tex]

\section{Sensor-Count Scaling}
\label{app:scaling}

\subsection{Architectural scaling}

Because each sensor is processed independently, local QCS stores and evolves a
constant-size $3\times3$ density matrix per sensor. The resulting quantum-state
cost therefore scales as $O(K)$ in sensor count, rather than as $O(9^K)$ for a
fully joint $K$-qutrit density matrix. This separates grid scale and sensor count from exponential Hilbert-space growth.

\subsection{Runtime and memory scaling}

We benchmark a vectorized implementation of Interleaved-QCS using synthetic
fields and untrained parameters; these measurements characterize computational
scaling only and are not accuracy results.

\begin{table}[h]
\centering
\caption{Interleaved-QCS inference cost versus sensor count.}
\label{tab:scaling-benchmark}
\begin{tabular}{lccc}
\toprule
$K$ & Inference time (200 samples) & Per-sensor cost & Propagator memory \\
\midrule
5    & 0.320s & 320.3\,\textmu s & 0.6 MB \\
20   & 0.177s & 44.2\,\textmu s  & 2.6 MB \\
100  & 0.514s & 25.7\,\textmu s  & 13.0 MB \\
500  & 0.587s & 5.9\,\textmu s   & 64.8 MB \\
1000 & 0.289s & 1.4\,\textmu s   & 129.6 MB \\
2000 & 0.434s & 1.1\,\textmu s   & 259.2 MB \\
\bottomrule
\end{tabular}
\end{table}

The measured memory cost grows approximately linearly with $K$, while batching
reduces per-sensor runtime at larger batch sizes.

\subsection{Accuracy versus sensor count}

To distinguish computational scaling from statistical performance, we train
Interleaved-QCS ($N=8$) on case118 CTA at
$K\in\{5,10,20,50,100\}$.

\begin{table}[h]
\centering
\caption{CTA detection performance versus sensor count on case118.}
\label{tab:accuracy-vs-k}
\begin{tabular}{lccc}
\toprule
$K$ & AP (exact) & AP (1000 shots) & Train time \\
\midrule
5   & 0.696 & 0.528 & 988s \\
10  & 0.731 & 0.697 & 2308s \\
20  & 0.692 & 0.668 & 6670s \\
50  & 0.705 & 0.672 & 14661s \\
100 & \textbf{0.793} & \textbf{0.778} & 9070s \\
\bottomrule
\end{tabular}
\end{table}

Performance is non-monotonic across $K$: increasing sensor count does not
systematically degrade detection, and the largest configuration tested achieves
the highest AP. The case118 regime is therefore harder than case14, but this
difficulty cannot be attributed simply to increasing $K$.
